# Supplementary material for: Debiased inference for a covariate-adjusted regression function
Source: arXiv:2210.06448 source file (2023-12-15)
Supplement: Supplementary file 1 [file consistency.tex]

\clearpage

\tw{We will no longer have a consistency result, but I'm leaving this here because the lemmas/analysis is probably useful.}

\paragraph{Proof of Theorem 1}
\textbf{Statement:} If \ref{cond:uniform_entropy_nuisances}--\ref{cond:cont_density} hold, then $|\theta_{n,h,b}(a_0)-\theta_0(a_0)|\inprob 0$.
\begin{proof}
For convenience, in this proof we omit the subscripts $h$, $b$. Lemma~\ref{lemma:first-order-decomposition} implies that
\begin{align*}
    |\theta_{n}(a_0) - \theta_{0}(a_0)|
    &\leq |\mathbb{P}_n \phi^*_{\infty, a_0} | +\sum_{j=1}^6|\mathrel{R}_{n, a_0, j}|.
\end{align*}
First, $|\mathbb{P}_n \phi^*_{\infty, a_0}| = \fasterthan(1)$ by weak law
of large numbers since it is an empirical mean of a fixed \tw{not fixed, depends on $h$} mean zero function.

\kt{I think this needs a bit more work since $F_n$, $\b{D}_n$ are random (but I need help here)}
By the central limit theorem for a fixed function with finite variance, $|\mathrel{R}_{n, h,b,a_0, 5}| = \bounded(n^{-1/2}) = \fasterthan(1)$.

In conclusion, we have shown that conditions \ref{cond:uniform_entropy_nuisances}--\ref{cond:cont_density} imply that $|\mathbb{P}_n \phi^*_{\infty, a_0}|$ as well as all six remainder terms are asymptotically negligible so that $|\theta_{n,h,b}(a_0)-\theta_0(a_0)| \inprob 0$ as we claimed.
\end{proof}

% We state the following property that becomes useful for later proofs using Lemma \ref{lm:phi_finite_moments}. Consider a class of functions $\s{F}_n^* =  \{(y,a,w) \mapsto h^{1/2}\phi^*_{\infty, h,b,a_0}(y,a,w) : a_0 \in \s{A}_0\}$ with an envelope function $F^*$. Using Lemma \ref{lm:phi_finite_moments} for $k=2$, we can show that 
% \begin{align*}
%     P_0|F|^2 \lesssim C h \implies P_0|F^*|^2 = \boundeddet(1)
% \end{align*}
% Thus, $||F^*||_{P_0, 2} = \boundeddet(1)$.
We now provide several supporting lemmas for proving the uniform consistency of $\theta_{n,h,b}(a_0)$.

\begin{lemma} \label{lm:covering_number}
We denote by $\s{G}_{\s{A}_0} := [\{w_{h,a_0,1}(a)K_{h,a_0}(a)-w_{b,a_0,3}(a)K_{b,a_0}(a)\}\eta(y,a,w) \,:\, a_0 \in \s{A}_0]$ a class of functions indexed by $\s{A}_0$, and by $G$ an envelope function. We also define an intrinsic semimetric $d$ such that
\begin{align*}
    d^2(s,t) := P_0[\{(w_{h,s,1}K_{h,s}-w_{b,s,3}K_{b,s})-(w_{h,t,1}K_{h,t}-w_{b,t,3}K_{b,t})\}\eta]^{2}.
\end{align*}
Assuming $P_0 \eta^2 < \infty$, then $ N(\varepsilon, \s{G}_{\s{A}_0}, d) \lesssim (h^2\varepsilon)^{-1}$.
\end{lemma}
\begin{proof}
By adding and subtracting terms and the triangular inequality, we have that 
\begin{align}
    d(s,t)=&\{P_0[\{(w_{h,s,1}K_{h,s}-w_{b,s,3}K_{b,s})-(w_{h,t,1}K_{h,t}-w_{b,t,3}K_{b,t})\}\eta]^{2}\}^{1/2}\nonumber\\
    &\leq [P_0\{(w_{h,s,1}K_{h,s}-w_{h,t,1}K_{h,t})\eta\}^2]^{1/2} + [P_0\{(w_{b,s,3}K_{b,s}-w_{b,t,3}K_{b,t})\eta\}^2]^{1/2}\nonumber\\
    &\leq [P_0\{(w_{h,s,1}K_{h,s}-w_{h,t,1}K_{h,s})\eta\}^2]^{1/2} + [P_0\{(w_{h,t,1}K_{h,s}-w_{h,t,1}K_{h,t})\eta\}^2]^{1/2}\nonumber\\
    &\qquad +[P_0\{(w_{b,s,3}K_{b,s}-w_{b,t,3}K_{b,s})\eta\}^2]^{1/2} + [P_0\{(w_{b,t,3}K_{b,s}-w_{b,t,3}K_{b,t})\eta\}^2]^{1/2}\label{eq:d_s_t}
\end{align}
The first summand of equation (\ref{eq:d_s_t}) can be further bounded as follows:
\begin{align*}
    &[P_0\{(w_{h,s,1}K_{h,s}-w_{h,t,1}K_{h,s})\eta\}^2]^{1/2} \\
    &= E_0\left(\int \left[h^{-1}\left\{\left(\frac{a-s}{h}\right)^j -\left(\frac{a-t}{h}\right)^j\right\} K\left(\frac{a-s}{h}\right)\eta(Y,a,W)\right]^2\, dF_0(a) \, \bigg| \, A=a\right)^{1/2}\\
    &= E_0\left(h^{-1}\int \left[\left\{u^j -\left(u+\frac{s-t}{h}\right)^j\right\} K(u)\eta(Y,s+uh,W)\right]^2 f_0(s+uh)\, du \, \bigg| \, A=s+uh\right)^{1/2}\\
    &\lesssim h^{-1/2}\left|\frac{s-t}{h}\right|^j \, \text{for } j = 0,1
\end{align*}
assuming $P_0 \eta^2 < \infty$ and $f_0$ is uniformly bounded over $\s{A}_0$. The second summand of equation (\ref{eq:d_s_t}) can be also bounded in terms of $|s-t|$ as follows:
\begin{align*}
    &[P_0\{(w_{h,t,1}K_{h,s}-w_{h,t,1}K_{h,t})\eta\}^2]^{1/2} \\
    &= E_0\left(\int \left[h^{-1}\left(\frac{a-t}{h}\right)^j  \left\{K\left(\frac{a-s}{h}\right)-K\left(\frac{a-t}{h}\right)\right\}\eta(Y,a,W)\right]^2\, dF_0(a) \, \bigg| \, A=a\right)^{1/2}\\
    &\lesssim h^{-1} E_0\left(\int_{-1}^1\left[u^j  \left|\frac{t-s}{h}\right|\eta(Y,t+uh,W)\right]^2f_0(t+uh)\, du \, \bigg| \, A=a\right)^{1/2}\\
    &\lesssim h^{-2}|s-t|.
\end{align*}
We use the Lipschitz continuity and compactness of the kernel over $[-1,1]$ to derive the first inequality. The remaining terms in equation (\ref{eq:d_s_t}) can  be bounded analogously as
$[P_0\{(w_{b,s,3}K_{b,s}-w_{b,t,3}K_{b,s})\eta\}^2]^{1/2} \lesssim h^{-1/2}\left|\frac{s-t}{h}\right|^j \, \text{for } j = 0,1,2,3$ and $[P_0\{(w_{b,t,3}K_{b,s}-w_{b,t,3}K_{b,t})\eta\}^2]^{1/2} \lesssim h^{-2}|s-t|$. 

Let $A_1, \dots A_K$ be intervals covering $\s{A}_0$ such that $\max_{1\leq j \leq K} |A_i| \leq \delta$. In order to cover $\s{A}_0$, we need at least $\delta^{-1}$ intervals. The results above implies that $\varepsilon \lesssim h^{-2}|\delta| + h^{-1/2}\left|\frac{\delta}{h}\right| + \dots + h^{-1/2}\left|\frac{\delta}{h}\right|^3$ (\kt{What should I do when $j=0$}) and the first summand requires the most $\varepsilon$-balls to cover $|\delta|$ as $\varepsilon \longrightarrow 0$ and $h \longrightarrow 0$ with the number proportional to $h^2\varepsilon$. Thus, the total number of $\varepsilon$-balls required to cover $\s{A}_0$ is bounded up to a constant by $(h^2\varepsilon)^{-1}$ as claimed.
\end{proof}

Next, we extend the earlier asymptotic equicontinuity results (i.e., Lemmas \ref{lm:stochastic_equicontinuity1} and \ref{lm:stochastic_equicontinuity2}) to sequences of stochastic processes so that they are also indexed by $\s{A}_0$. 
First, we consider the following sequence of stochastic processes $\s{V}_{n, h, j} := \left\{ V_{n, h, j}(a, \eta) : a\in \s{A}_0, \eta \in \s{H}\right\}$ indexed by a set of functions $\s{H} = \{\eta : \s{Y}\times \s{A} \times\s{W} \mapsto \d{R}\}$:
\[V_{n, h, j}(a_0, \eta) = \left(\frac{h}{\log 1/h}\right)^{1/2}  \left(\frac{a-a_0}{h}\right)^{j-1}\frac{1}{h}K\left(\frac{a-a_0}{h}\right) \eta(y, a, w).\]
We then state the following lemma;
\kt{If we omit consistency results, we do not need the following results (we still need similar lemmas but with faster rates of convergence)}
\begin{lemma}\label{lm:sup_stochastic_equicontinuity1}
Suppose \ref{cond:bounded_K}--\ref{cond:cont_density} hold for all $a_0 \in \s{A}_0$. If $\s{H}$ satisfies the uniform-entropy condition (\ref{cond:uniform_entropy_condition}) and $\sup_{\eta\in \s{H}}P_0|\eta|^{2+\delta} < \infty$, then for any $\eta_1, \eta_2 \in \s{H}$ such that $\sup_{a_0 \in \s{A}_0}\rho_{a_0, \varepsilon}(\eta_1, \eta_2)=\fasterthan(1)$,  $\sup_{a_0 \in \s{A}_0}\d{G}_n \{V_{n, h, j}(a_0, \eta_1)-V_{n, h, j}(a_0, \eta_2)\}= \fasterthan(1)$ for $j = 1,2,3,4$.
\end{lemma}
\begin{proof}
\kt{TODO: We cannot use asymptotic equicontinuity for this proof?}
\end{proof}

Next, we consider the following sequence of stochastic processes $\s{W}_{n, h, j} := \left\{ W_{n, h, j}(a, \omega) : a\in \s{A}, \omega \in \Omega \right\}$ indexed by a set of functions $\Omega = \{\omega : \s{A} \times\s{W} \mapsto \d{R}\}$ uniformly bounded by some constant $C < \infty$ such that $|\omega| \leq C$ for all $\omega \in \Omega$:
\[W_{n, h, j}(a_0, \eta) = \left(\frac{1}{\log 1/h}\right)^{1/2}\int \omega(a, w)\left(\frac{a-a_0}{h}\right)^{j-1}h^{-1}K\left(\frac{a-a_0}{h}\right)\, dF_0(a).\]
We then state the following lemma;
\begin{lemma}\label{lm:sup_stochastic_equicontinuity2}
Suppose \ref{cond:bounded_K}--\ref{cond:cont_density} hold for all $a_0 \in \s{A}_0$. If $\Omega$ satisfies the uniform-entropy condition (\ref{cond:uniform_entropy_condition}), then for any $\omega_1, \omega_2 \in \Omega$ such that $\sup_{a_0 \in \s{A}_0}\rho_{a_0, \varepsilon}(\omega_1, \omega_2)=\fasterthan(1)$,  $\sup_{a_0 \in \s{A}_0}\d{G}_n \{W_{n, h, j}(a_0, \omega_1)-W_{n, h, j}(a_0, \omega_2)\}= \fasterthan(1)$ for $j = 1,2,3,4$. 
\end{lemma}
\begin{proof}
\kt{TODO: We cannot use asymptotic equicontinuity for this proof?}
\end{proof}
\paragraph{Proof of Theorem 2}
\textbf{Statement:}
If \ref{cond:uniform_entropy_nuisances}--\ref{cond:cont_density} hold for all $a_0 \in \s{A}_0$ and $\log n / nh = \fasterthandet(1)$, then $\sup_{a_0\in \s{A}_0}|\theta_{n,h,b}(a_0)-\theta_0(a_0)|\inprob 0$

\begin{proof}
The first-order decomposition of the estimator from Lemma \ref{lemma:first-order-decomposition} implies that
\begin{align*}
    \sup_{a_0\in\s{A}_0}\left|\theta_{n,h,b}(a_0) - \theta_{0}(a_0)\right|
    &\leq  \sup_{a_0\in\s{A}_0}\left|\mathbb{P}_n \phi^*_{\infty, a_0} \right| +\sum_{j=1}^6 \sup_{a_0\in\s{A}_0}\left|\mathrel{R}_{n, h,b,a_0, j}\right|.
\end{align*}
In what follows, we claim that $\left|\mathbb{P}_n \phi^*_{\infty, a_0} \right|$ and all remainder terms tend to zero uniformly over $\s{A}_0$. We omit the subscripts $h$ and $b$ from $\Gamma$ and $\gamma$ when it is clear.

First, we can further bound $\sup_{a_0\in\s{A}_0}\left|\mathbb{P}_n \phi^*_{\infty, a_0} \right|$ by adding and subtracting $\d{P}_n(\Gamma_{0,a_0}\theta_0)$ as follows:
\begin{align}
    \sup_{a_0\in\s{A}_0}\left|\d{P}_n \phi^*_{\infty, h, b, a_0}\right|&\leq \sup_{a_0\in\s{A}_0}\left|\d{P}_n\Gamma_{0,a_0} (\xi_\infty - \theta_0)\right| +\sup_{a_0\in\s{A}_0}\left|\d{P}_n(\Gamma_{0,a_0} \theta_0-\gamma_{0,a_0} )\right|\nonumber\\
    &\qquad\qquad+ \sup_{a_0\in\s{A}_0}\left|\d{P}_n\left\{ \int\Gamma_{0,a_0} \left( \mu_\infty - \int \mu_\infty \, dQ_0 \right) \, dF_0 \right\}\right|\label{eq:sup_phi_consistency}
\end{align}
We control the first term in display (\ref{eq:sup_phi_consistency}) using Theorem 2.14.1 of \cite{vandervaart1996}. We define a class of functions $\s{G}_{\s{A}_0}$ indexed by $\s{A}_0$ as follows:
\[\s{G}_{\s{A}_0} := \left\{(y,a,w) \mapsto h^{1/2}\left(\frac{a-a_0}{h}\right)^{j-1}\frac{1}{h}K\left(\frac{a-a_0}{h}\right)\{\xi_\infty(y,a,w)-\theta_0(a)\}: a_0 \in \s{A}_0\right\}\]
and denote by $G$ an envelop function for $\s{G}_{\s{A}_0}$. First, we claim that $||G||_{P_0, 2} = \boundeddet(1)$. By the change of variables, we have that 
\begin{align*}
   ||G_{\s{A}_0}||_{P_0, 2}^2 = &\sup_{a_0 \in \s{A}_0} E_0 \left[\left|h^{1/2}\left(\frac{a-a_0}{h}\right)^{j-1}\frac{1}{h}K\left(\frac{a-a_0}{h}\right)\{\xi_\infty(y,a,w)-\theta_0(a)\}\right|^2\right] \\
    &\leq \sup_{a_0 \in \s{A}_0}\left(P_0|\xi_\infty|^2 + P_0|\theta_0|^2 \right)\sup_{a_0\in\s{A}}f_0(a_0)\int |u|^{2(j-1)}K^2(u)  \, du.
\end{align*}
In view of condition \ref{cond:uniform_entropy_nuisances} and $E_0 |Y|^2 < \infty$, we conclude that $P_0\xi^2_\infty$ and $P_0\theta^2_0$ are both bounded and thus $||G||_{P_0, 2} = \boundeddet(1)$. Next, we let $\eta(y,a,w) := \xi_\infty(y,a,w) - \theta_0(a)$ then it follows that $P_0 \eta^2 < \infty$. By Lemma \ref{lm:covering_number}, the $\varepsilon$-covering number for $\s{G}_{\s{A}_0}$ is proportional to $(h^{3/2}\varepsilon)^{-1}$ and the uniform entropy is bounded up to a constant by $\{\log n\}^{1/2}$ provided $h = \boundeddet(n^{-\omega})$ for some $\omega > 0$. Now we use Theorem 2.14.1 of \cite{vandervaart1996} to obtain that 
\[E_0 \left(\sup_{g_{a_0} \in \s{G}_{\s{A}_0}}\left|\d{G}_n g_{a_0} \right|\right) = \boundeddet\left(\{\log n\}^{1/2}\right).\]
Additionally, Lemma \ref{lm:D0_altform} implies that $\sup_{a_0\in\s{A}_0}\left|\b{D}_{0,h,a_0}^{-1}\right|$ and $\sup_{a_0\in\s{A}_0}\left|\b{D}_{0,b,a_0}^{-1}\right|$ are $\boundeddet(1)$ provided that $f_0$ is uniformly bounded away from zero. In view of these results, we conclude that 
\begin{align*}
    &\sup_{a_0\in\s{A}_0}\left|\d{G}_nh^{1/2}\Gamma_{0,a_0} (\xi_\infty - \theta_0)\right| = \boundeddet(\{\log n\}^{1/2})\\
    &\implies \sup_{a_0\in\s{A}_0}\left|\d{P}_n\Gamma_{0,a_0} (\xi_\infty - \theta_0)\right| = \boundeddet(\{\log n/nh\}^{1/2})
\end{align*}
which tends to zero provided $\log n/nh = \fasterthandet(1)$.

For the second term in display (\ref{eq:sup_phi_consistency}), we recall the proof of Lemma \ref{lm:lindeberg_feller_CLT} in which we establish that for each $a_0 \in \s{A}_0$,
\[\Gamma_{0,a_0} \theta_0(a)-\gamma_{0,a_0}(a) = e_1^T \b{D}_{0,h,a_0}^{-1} w_{h,a_0,1}(a) K_{h,a_0}(a)\fasterthandet(h) +e_3^T c_2 \tau^2 \b{D}_{0,b,a_0}^{-1}w_{b,a_0,3}(a) K_{b,a_0}(a)\fasterthandet(b^3).\]
The remainder terms in the above display, $\fasterthandet(h)$ and $\fasterthandet(b^3)$, derive from Taylor series approximation of $\theta_0$ at $a_0$. Thus, the preceding display holds uniformly over $\s{A}_0$ assuming $\theta_0$ is at least twice differentiable at all $a_0 \in \s{A}_0$. We also recall that $P_0(\Gamma_{0,a_0}-\gamma_{0,a_0})=0$ for each $a_0 \in \s{A}_0$, and thus the second summand in equation (\ref{eq:sup_phi_consistency}) can be bounded as follows:
\begin{align*}
    \sup_{a_0 \in \s{A}_0}\left|(\d{P}_n-P_0)(\Gamma_{0,a_0} \theta_0-\gamma_{0,a_0})\right| &\leq \sup_{a_0 \in \s{A}_0}\left| e_1^T \b{D}_{0,h,a_0}^{-1} (\d{P}_n-P_0)w_{h,a_0,1} K_{h,a_0}\fasterthandet(h) \right|\\
    &\qquad+\sup_{a_0 \in \s{A}_0}\left| e_3^T c_2 \tau^2 \b{D}_{0,b,a_0}^{-1} (\d{P}_n-P_0)w_{b,a_0,3} K_{b,a_0}\fasterthandet(b^3)\right|.
\end{align*}
First, $\sup_{a_0 \in \s{A}_0}\left|\b{D}_{0,h,a_0}^{-1}\right|$ and $\sup_{a_0 \in \s{A}_0}\left| \b{D}_{0,b,a_0}^{-1}\right|$ are both $\boundeddet(1)$ assuming $f_0$ is uniformly bounded away from zero. Also, Theorem 2.3 by \cite{gine2002} implies that $\sup_{a_0 \in \s{A}_0}|(\d{P}_n-P_0)w_{h,a_0,1} K_{h,a_0}|$ and $\sup_{a_0 \in \s{A}_0}|(\d{P}_n-P_0)w_{b,a_0,3} K_{b,a_0}|$ are $\bounded(\{\log n /nh\}^{1/2})$. We thus claim that the second summand of equation (\ref{eq:sup_phi_consistency}) is $\fasterthan(1)$.

For the third summand, we establish that $\{w \mapsto \int \Gamma_{0,a_0}(a) \mu_\infty(a,w) \, dF_0(a): a_0 \in \s{A}_0\}$ is $P_0$-Donsker using Lemma 7 of \cite{westling2018causal} in view of the uniform boundedness of $\Gamma_{0,a_0}$ and $\mu_\infty$ \kt{Can I use this? This is only true for $h > 0$}. Therefore, we have that $\sup_{a_0 \in \s{A}_0}|(\d{P}_n - P_0)\int \Gamma_{0,a_0}(a) \mu_\infty(a,w) \, dF_0(a)| = \bounded(n^{-1/2})$ and thus $\sup_{a_0\in\s{A}_0}\left|\d{P}_n \phi^*_{\infty, h, b, a_0}\right| \inprob 0$ . 

Now we turn to six remainder terms. First, Lemma \ref{lm:asymptotic_bias} implies $\sup_{a_0 \in \s{A}_0}|\mathrel{R}_{n, h,b,a_0, 1}|=\boundeddet(h^{2+\delta})$ for some $\delta \in (0, 2]$ provided \ref{cond:doubly_robust}--\ref{cond:cont_density} hold for all $a_0 \in \s{A}_0$ and hence $\sup_{a_0 \in \s{A}_0}|\mathrel{R}_{n, h,b,a_0, 1}| \inprob 0$.

Next, we can uniformly bound $|\mathrel{R}_{n, h,b,a_0, 2}|$ as follows:
\begin{align*}
    \sup_{a_0 \in \s{A}_0}|\mathrel{R}_{n, h,b,a_0, 2}| &\leq \sup_{a_0 \in \s{A}_0}\left|(\d{P}_n - P_0)   \Gamma_{0,a_0} \left\{\left( \psi_n + \int \mu_n  \, dQ_0\right)-\left( \psi_\infty + \int \mu_\infty  \, dQ_0\right)\right\}\right| \\&
    \qquad + \sup_{a_0 \in \s{A}_0}\left|(\d{P}_n - P_0) \int \Gamma_{0,a_0} (\mu_n - \mu_\infty) \, dF_0  \right|.
\end{align*}
We use the asymptotic equcontinuity results (i.e., Lemmas \ref{lm:sup_stochastic_equicontinuity1} and \ref{lm:sup_stochastic_equicontinuity2}) to control the terms above. First, $\sup_{a_0 \in \s{A}_0}\left|\b{D}_{0,h,a_0}^{-1}\right|$ and $\sup_{a_0 \in \s{A}_0}\left|\b{D}_{0,b,a_0}^{-1}\right|$ are both $\boundeddet(1)$ provided $f_0$ is uniformly bounded away from zero. Then, we use Lemma \ref{lm:sup_stochastic_equicontinuity1} to control the first term in the preceding display. As we have established in the proof of Theorem 2, a class of functions $\left\{(y,a,w) \mapsto \psi(y,a,w) + \int \mu(a,w) \, dQ_0(w) : \mu \in \s{F}_\mu, g \in \s{F}_g \right\}$ is $P_0$-Donsker. In view of this result and condition \ref{cond:limiting_nuisances} holding uniformly over $\s{A}_0$, we conclude that the first term in display is $\fasterthan(\{\log n / nh\}^{1/2})$ by Lemma \ref{lm:sup_stochastic_equicontinuity1} since \begin{align*}
    &\sup_{a_0 \in \s{A}_0}\left|\d{G}_n   \left(\frac{h}{\log 1/h}\right)^{1/2}  \Gamma_{0,a_0} \left\{\left( \psi_n + \int \mu_n  \, dQ_0\right)-\left( \psi_\infty + \int \mu_\infty  \, dQ_0\right)\right\}\right| = \fasterthan(1)\\
    &\qquad \implies \sup_{a_0 \in \s{A}_0}\left|(\d{P}_n - P_0) \Gamma_{0,a_0} \left\{\left( \psi_n + \int \mu_n  \, dQ_0\right)-\left( \psi_\infty + \int \mu_\infty  \, dQ_0\right)\right\}\right| = \fasterthan(\{\log n/nh\}^{1/2}).
\end{align*}
Similarly, we use Lemma \ref{lm:sup_stochastic_equicontinuity2} to control the second term in the preceding display. As established $\s{F}_\mu$ is $P_0$-Donsker and assuming \ref{cond:limiting_nuisances} uniformly for all $a_0 \in \s{A}_0$, and thus we conclude that the second term in display is $\fasterthan(\{\log n / n\}^{1/2})$, which tends to zero for large $n$.

Next, we bound $\sup_{a_0 \in \s{A}_0}|\mathrel{R}_{n, h, b, a_0, 3}|$ by the sum of empirical processes such that 
\begin{align}
    \sup_{a_0 \in \s{A}_0}|\mathrel{R}_{n, h, b, a_0, 3}|&\leq \sup_{a_0 \in \s{A}_0}\left|(\d{P}_n - P_0) \left[ \left(\Gamma_{n,a_0} - \Gamma_{0,a_0}\right)\left\{\left( \psi_n + \int \mu_n \, dQ_0 \right) -\left( \psi_\infty + \int \mu_\infty \, dQ_0 \right)\right\}\nonumber\right.\right.\\
    &\qquad\qquad\qquad\qquad+ \left.\left.\int \left(\Gamma_{n,a_0} - \Gamma_{0,a_0}\right) (\mu_n-\mu_\infty) \, dF_0 \right]\right|\nonumber\\
    &\qquad+\sup_{a_0 \in \s{A}_0}\left|(\d{P}_n - P_0) \left\{ \left(\Gamma_{n,a_0} - \Gamma_{0,a_0}\right)\left( \psi_\infty + \int \mu_\infty \, dQ_0 \right) + \int \left(\Gamma_{n,a_0} - \Gamma_{0,a_0}\right) \mu_\infty \, dF_0 \right\}\right|. \label{eq:sup_consistency_R2_decomposition}
\end{align}
By an analogous argument to the proof of Theorem 2, the first term in the preceding display can be summarized as the sum of products of empirical processes as follows:
\begin{align*}
    &\sup_{a_0 \in \s{A}_0}\left|(\d{P}_n - P_0) \left[ \left(\Gamma_{n,a_0} - \Gamma_{0,a_0}\right)\left\{\left( \psi_n + \int \mu_n \, dQ_0 \right) -\left( \psi_\infty + \int \mu_\infty \, dQ_0 \right)\right\}\nonumber\right.\right.+ \left.\left.\int \left(\Gamma_{n,a_0} - \Gamma_{0,a_0}\right) (\mu_n-\mu_\infty) \, dF_0 \right]\right|\nonumber\\
    &\qquad\leq\sup_{a_0 \in \s{A}_0}\left|e_1^T\left(\b{D}_{n,h,a_0}^{-1}-\b{D}_{0,h,a_0}^{-1}\right)(\d{P}_n - P_0) w_{h,a_0,1} K_{h,a_0} \left\{\left( \psi_n + \int \mu_n \, dQ_0 \right) -\left( \psi_\infty + \int \mu_\infty \, dQ_0 \right)\right\}\right|\nonumber\\
    &\qquad\qquad + \sup_{a_0 \in \s{A}_0}\left|c_2 \tau^2 e_3^T\left(\b{D}_{n,b,a_0}^{-1}-\b{D}_{0,b,a_0}^{-1}\right)(\d{P}_n - P_0) w_{b,a_0,3} K_{b,a_0} \left\{\left( \psi_n + \int \mu_n \, dQ_0 \right) -\left( \psi_\infty + \int \mu_\infty \, dQ_0 \right)\right\}\right|\nonumber\\
    &\qquad\qquad + \sup_{a_0 \in \s{A}_0}\left|e_1^T\left(\b{D}_{n,h,a_0}^{-1}-\b{D}_{0,h,a_0}^{-1}\right)(\d{P}_n - P_0) \int w_{h,a_0,1} K_{h,a_0} (\mu_n-\mu_\infty) \, dF_0\right|\nonumber\\
    &\qquad \qquad+ \sup_{a_0 \in \s{A}_0}\left|c_2 \tau^2 e_3^T\left(\b{D}_{n,b,a_0}^{-1}-\b{D}_{0,b,a_0}^{-1}\right)(\d{P}_n - P_0) \int w_{b,a_0,3} K_{b,a_0} (\mu_n-\mu_\infty) \, dF_0\right|
\end{align*}
The rates of $\sup_{a_0 \in \s{A}_0}\left|\b{D}_{n,h,a_0}^{-1}-\b{D}_{0,h,a_0}^{-1}\right|$ and $\sup_{a_0 \in \s{A}_0}\left|\b{D}_{n,b,a_0}^{-1}-\b{D}_{0,b,a_0}^{-1}\right|$ are provided by Theorem 2.3 of \cite{gine2002} as $\bounded(\{\log n / nh\}^{1/2})$. Additionally, since all suitable conditions for Lemma \ref{lm:sup_stochastic_equicontinuity1} are satisfied by the argument for controlling $\sup_{a_0 \in \s{A}_0}\left|\mathrel{R}_{n, h, b, a_0, 2}\right|$, the empirical process term from the first two summands are $\fasterthan(\{\log n/ nh\}^{1/2})$ and thus they are $\fasterthan(\log n/nh)$, which tends to zero for large $n$.

Next, the second component of equation (\ref{eq:sup_consistency_R2_decomposition}) can be bounded as follows:
\begin{align}
    &\sup_{a_0\in \s{A}_0}\left|(\d{P}_n - P_0) \left\{ \left(\Gamma_{n,a_0} - \Gamma_{0,a_0}\right)\left( \psi_\infty + \int \mu_\infty \, dQ_0 \right) + \int \left(\Gamma_{n,a_0} - \Gamma_{0,a_0}\right) \mu_\infty \, dF_0 \right\}\right|\nonumber\\
    &\qquad\leq\sup_{a_0\in \s{A}_0}\left|e_1^T\left(\b{D}_{n,h,a_0}^{-1}-\b{D}_{0,h,a_0}^{-1}\right)(\d{P}_n - P_0) w_{h,a_0,1} K_{h,a_0} \left( \psi_\infty + \int \mu_\infty \, dQ_0 \right)\right|\nonumber\\
    &\qquad\qquad + \sup_{a_0\in \s{A}_0}\left|c_2 \tau^2 e_3^T\left(\b{D}_{n,b,a_0}^{-1}-\b{D}_{0,b,a_0}^{-1}\right)(\d{P}_n - P_0) w_{b,a_0,3} K_{b,a_0} \left( \psi_\infty + \int \mu_\infty \, dQ_0 \right)\right|\nonumber\\
    &\qquad\qquad + \sup_{a_0\in \s{A}_0}\left|e_1^T\left(\b{D}_{n,h,a_0}^{-1}-\b{D}_{0,h,a_0}^{-1}\right)(\d{P}_n - P_0) \int w_{h,a_0,1} K_{h,a_0} \mu_\infty \, dF_0\right|\nonumber\\
    &\qquad\qquad + \sup_{a_0\in \s{A}_0}\left|c_2 \tau^2 e_3^T\left(\b{D}_{n,b,a_0}^{-1}-\b{D}_{0,b,a_0}^{-1}\right)(\d{P}_n - P_0) \int w_{b,a_0,3} K_{b,a_0} \mu_\infty \, dF_0\right|. \label{eq:14}
\end{align}
Now we apply Theorem 2.14.1 of \cite{vandervaart1996} to classes of functions indexed by $\s{A}_0$. We denote by $\s{G}_{\s{A}_0}$ $\{(y,a,w) \mapsto h^{1/2}w_{h,a_0,1} K_{h,a_0} ( \psi_\infty + \int \mu_\infty \, dQ_0)\,:\, a_0 \in \s{A}_0\}$ and $G$ its envelope. We can show that $||G||_{P_0, 2} < \infty$ by the change of variables and condition \ref{cond:uniform_entropy_nuisances} as well as $E_0 Y^2 < \infty$. Also let $\eta(y,a,w) := \psi_\infty(y,a,w) + \int \mu_\infty(a,w) \, dQ_0(w)$. Since $P_0 \eta^2 < \infty$, Lemma \ref{lm:covering_number} implies that the $\varepsilon$-covering number of $\s{G}_{\s{A}_0}$ is proportional to $(h^{3/2}\varepsilon)^{-1}$. Therefore, Theorem 2.14.1 of \cite{vandervaart1996} implies that 
\begin{align*}
    \sup_{a_0\in\s{A}_0}(\d{P}_n - P_0) w_{h,a_0,1} K_{h,a_0} \left( \psi_\infty + \int \mu_\infty \, dQ_0 \right) = \bounded(\{\log n /nh\}^{1/2}).
\end{align*}
Hence the first summand in (\ref{eq:14}) is $\bounded(\log n/nh)$ which tends to zero assuming $\log n/nh = \fasterthandet(1)$. The second summand in (\ref{eq:14}) is also $\bounded(\log n/nh)$ by an analogous argument. Next, we define a class of functions $\s{H}_{\s{A}_0} := \{w \mapsto \int w_{h,a_0,1} K_{h,a_0} \mu_\infty \, dF_0\}$ and let $H$ be its envelope. Then, we can show $||H||_{P_0, 2} < \infty$ by the change of variables as well as the condition \ref{cond:uniform_entropy_nuisances}. To show the uniform entropy bound, we first note that 
\begin{align*}
    &\left\{E_0 \left(\int w_{h,s,1} K_{h,s} \mu_\infty \, F_0-\int w_{h,t,1} K_{h,t} \mu_\infty\, F_0\right)^2\right\}^{1/2} \\
    &= \left\{E_0 \left(\int u^{j-1}K(u)\mu_\infty(s+uh, w) \, f_0(s+uh)\, du-\int u^{j-1}K(u)\mu_\infty(t+uh, w) \, f_0(t+uh)\, du\right)^2\right\}^{1/2} \\
    &\lesssim |s-t|
\end{align*}
assuming there exists moduli of continuity for $\mu_\infty$ and $f_0$. Thus, the covering number is proportional to $\varepsilon^{-1}$ which can be bounded by $n$ for $n$ large enough since $\s{A}_0$ is compact. We therefore conclude that the uniform entropy bound for $\s{H}_{\s{A}_0}$ is bounded up to a constant by $\{\log n\}^{1/2}$. Hence by Theorem 2.14.1 of \cite{vandervaart1996}, we have that
\begin{align*}
    \sup_{a_0\in \s{A}_0}\left|e_1^T\left(\b{D}_{n,h,a_0}^{-1}-\b{D}_{0,h,a_0}^{-1}\right)(\d{P}_n - P_0) \int w_{h,a_0,1} K_{h,a_0} \mu_\infty \, dF_0\right| = \bounded(\{\log n / n\}^{1/2})
\end{align*}
which tends to zero as $n \longrightarrow \infty$. The last term in (\ref{eq:14}) can be controlled analogously and thus we conclude that $\sup_{a_0\in\s{A}}|\mathrel{R}_{n,h,b,a_0, 3}| = \fasterthan(1)$ Additionally, Lemma \ref{lm:u-process} implies that $ \sup_{a_0\in\s{A}_0}|\mathrel{R}_{n,h,b,a_0, 4}| = \fasterthan(1)$ provided $\log n / nh= \fasterthandet(1)$.

For $\sup_{a_0\in\s{A}_0}|\mathrel{R}_{n,h,b,a_0, 5}|$, we can write that
\begin{align*}
    \sup_{a_0\in\s{A}_0}|\mathrel{R}_{n,h,b,a_0, 5}| &\leq \iint_{\s{S}_1}  \sup_{a_0\in\s{A}_0}|\Gamma_{n,a_0}(a)||\mu_n(a,w) - \mu_\infty(a,w)|\left|1-\frac{g_0(a,w)}{g_n(a,w)}\right|dF_0(a)dQ_0(w)\\
    &\qquad +\iint_{\s{S}_2}  \sup_{a_0\in\s{A}_0}|\Gamma_{n,a_0}(a)||\mu_n(a,w) - \mu_0(a,w)|\left|1-\frac{g_\infty(a,w)}{g_n(a,w)}\right|dF_0(a)dQ_0(w)\\&
    \qquad+\iint_{\s{S}_3}  \sup_{a_0\in\s{A}_0}|\Gamma_{n,a_0}(a)||\mu_n(a,w) - \mu_\infty(a,w)|\left|1-\frac{g_\infty(a,w)}{g_n(a,w)}\right|dF_0(a)dQ_0(w)\\
    &\lesssim  \sup_{a_0\in\s{A}_0}\{P_0(\mu_n-\mu_\infty)^2P_0(1-g_0/g_n )^2\}^{1/2} +  \sup_{a_0\in\s{A}_0}\{P_0(\mu_n-\mu_0)^2P_0(1-g_\infty/g_n )^2\}^{1/2}\\&\qquad
    +  \sup_{a_0\in\s{A}_0}\{P_0(\mu_n-\mu_\infty)^2P_0(1-g_\infty/g_n )^2\}^{1/2}
\end{align*}
By assumption, $P_0(\mu_n - \mu_\infty) = \fasterthan(1)$, and since $g_n$ is bounded uniformly above and away from zero, $P_0(1-g_\infty/g_n)^2 = \fasterthan(1)$. Also, $P_0(\mu_n - \mu_0)^2 = \bounded(1)$ and $P_0(1-g_0/g_n)^2 = \bounded(1)$ since $\mu_n$, $g_n$, $\mu_0$ and $g_0$ all belong to the class of bounded functions. Hence $\sup_{a_0\in\s{A}_0}|\mathrel{R}_{n,h,b,a_0, 5}| = \fasterthan(1)$.

Finally, $\mathrel{R}_{n, h,b, a_0, 6}$ can be uniformly bounded by two terms as follows:
\begin{align*}
    \sup_{a_0 \in \s{A}_0}|\mathrel{R}_{n, h,b, a_0, 6}| &\leq \sup_{a_0 \in \s{A}_0}e_1^T\left| \b{D}_{0,h, a_0} - \b{D}_{n,h, a_0}\right|\sup_{a_0 \in \s{A}_0}e_1^T\left| \b{D}^{-1}_{n,h, a_0} - \b{D}^{-1}_{0,h, a_0}\right|\sup_{a_0 \in \s{A}_0}\left|e_1^T \b{D}^{-1}_{0,h, a_0} P_0 \left( w_{h,a_0, 1} K_{1, a_0} \theta_0\right)\right| \\
    &\qquad+ \sup_{a_0 \in \s{A}_0}e_3^T\left| \b{D}_{b, a_0, 3} - \b{D}_{n,b, a_0} \right|\sup_{a_0 \in \s{A}_0}e_3^T\left| \b{D}^{-1}_{n,b, a_0} - \b{D}^{-1}_{0,b, a_0}\right|\sup_{a_0 \in \s{A}_0}\left|e_3^T c_2 \tau^2 \b{D}^{-1}_{0,b, a_0} P_0 \left( w_{b,a_0, 3} K_{b, a_0} \theta_0\right)\right|
\end{align*}
We first note that both $\sup_{a_0 \in \s{A}_0}\left|e_1^T \b{D}^{-1}_{0,h, a_0} P_0 \left( w_{h,a_0, 1} K_{1, a_0} \theta_0\right)\right|$ and $\sup_{a_0 \in \s{A}_0}\left|e_3^T c_2 \tau^2 \b{D}^{-1}_{0,b, a_0} P_0 \left( w_{b,a_0, 3} K_{b, a_0} \theta_0\right)\right|$ are $\bounded(1)$ in view of the uniform boundedness of $\mu_0$ and $1/f_0$. Also the leading terms are both $\bounded(\{\log n / nh\}^{1/2})$ based on Theorem 2.3 of \cite{gine2002}. We thus have that $\sup_{a_0 \in \s{A}_0}|\mathrel{R}_{n, h,b, a_0, 6}| = \bounded(\log n / nh)$ and thus tends to zero provided $\log n /nh = \fasterthandet(1)$. 
\end{proof}
