# Supplementary material for: Debiased inference for a covariate-adjusted regression function
Source: arXiv:2210.06448 source file (2023-12-15)
Supplement: Supplementary file 2 [file localmax.tex]

\clearpage

\section{Local Maximal Inequality}

Our goal is to show $\sup_{a_0 \in \s{A}_0}\mathrel{R}_{n, h,b,a_0, 2} = \fasterthan(\{nh \log n\}^{-1/2})$. In particular, we focus on two terms that arise in the following decomposition:
\begin{align}
    &\sup_{a_0 \in \s{A}_0}(nh\log n)^{1/2}\mathrel{R}_{n, h,b,a_0, 2} \nonumber\\
    &= \sup_{a_0 \in \s{A}_0}\d{G}_n\left\{ (h\log n)^{1/2} \Gamma_{0,h,b,a_0} \left( \psi_n - \psi_\infty \right) \right\} + \sup_{a_0 \in \s{A}_0}\d{G}_n\left\{ (h\log n)^{1/2} \Gamma_{0,h,b,a_0} \left( \int \mu_n \, dQ_0 - \int \mu_\infty \, dQ_0 \right) \right\} + \dots \nonumber
\end{align}

$(h^{-j} \log n) \d{G}_n(\eta_{s,\lambda_n} - \eta_{s,\lambda})$

If $\rho(\lambda_n, \lambda_\infty) \leq r_n$ almost surely as $n \to \infty$, then
\[E\left[\left| \d{G}_n(\eta_{s,\lambda_n} - \eta_{s,\lambda_\infty}) \right| \right] \leq E\left[ \sup_{\gamma \in \s{H}_{r_n}} \left| \d{G}_n \gamma\right| \right]\]
where 
\[ \s{H}_{r} := \{\eta_{s,\lambda} - \eta_{s,\lambda_\infty} : \lambda \in \Lambda, \rho(\lambda, \lambda_\infty) \leq r, s \in \s{S} \}. \] 

Suppose $\s{H}_\infty$ has envelope function $H$
If $\sup_Q \log N(\varepsilon \| H\|_{Q,2}, \s{H}_\infty, L_2(Q)) \leq C \varepsilon^{-V}$ for $V<2$ then
\[ J(\delta, \s{H}_\infty, H) \leq \int_0^\delta \sqrt{1 + C \varepsilon^{-V}} \, d\varepsilon \lesssim \int_0^\delta  \varepsilon^{-V/2} \, d\varepsilon  \lesssim \delta^{1-V/2}\]

We consider the sequence of stochastic processes $\{V_n(s, \lambda) : s\in \s{S}, \lambda \in \Lambda\}$, for $V_n(s, \lambda) := \d{G}_n \eta_{h,s, j,\lambda}$, where
\[\eta_{h,s, j,\lambda}(y,a,w) := (h\log n)^{1/2} \left(\frac{a-s}{h}\right)^{j-1}K_{h,s}(a) (\lambda-\lambda_\infty)(y, a, w).\]
We assume that $\lambda_\infty$ is fixed and $\s{S}$ is compact. We also work with the following semi-metric on $\Lambda$:
\[ \rho(\lambda_1, \lambda_2) := \sup_{s \in \s{S}} \left(E_0 \left[ \left\{ \lambda_1(Y,A,W) - \lambda_2(Y,A,W) \right\}^2 \mid A = s \right] \right)^{1/2}.\] 
We now study the class $\s{H}_{h,s,r,j} := \{ \eta_{h,s, j,\lambda} : s \in \s{S}, \lambda \in \Lambda_r\}$ where $\Lambda_r$ denotes a set of all functions in $\Lambda$ within the $\rho$-ball of radius $r$ around $\lambda_\infty$, or $\Lambda_r := \{\lambda \in \Lambda : \rho(\lambda, \lambda_\infty) \leq r\}$ ($r$ also depends on $n$).
\begin{lemma} \label{lm:uniform_entropy}
If $\sup_Q \log N(\varepsilon, \Lambda, L_2(Q)) \leq C \varepsilon^{-V}$ for some $C < \infty$ and $V < 2$, then 
$J(\delta, \s{H}_{h,s,r,j},L_2) \leq C'\delta^{1-V/2}$ for some $C' < \infty$. 
\end{lemma}
\begin{proof}[\bfseries{Proof of Lemma}]
Our first aim is to bound the uniform entropy of $\s{H}_{h,s,r,j}$. We introduce the following classes of functions:
\begin{align*}
    \s{H}_{h} := \left\{ (h\log n)^{1/2} K_{h,s}(a) : s \in \s{S}\right\}, \s{H}_{j} := \left\{\left(\frac{a-s}{h}\right)^{j-1}I\left(\left|\frac{a-s}{h}\right|\leq 1\right)  : s \in \s{S}\right\} \, \text{ and } \s{H}_{r} := \left\{ (\lambda - \lambda_\infty)(y,a,w) :  \lambda \in \Lambda_r \right\}. 
\end{align*}
Then Lemma~5.1 of~\cite{vanderVaartvanderLaan2006} implies that 
\begin{align}
    &\sup_Q  N\left(\varepsilon \| H_{h,s,j}\|_{Q,2}, \s{H}_{h,s,r,j}, L_2(Q) \right) \nonumber\\
    &\leq \sup_Q N\left(\varepsilon \| H_{h}\|_{Q,2}, \s{H}_{h}, L_2(Q) \right)\sup_Q N\left(\varepsilon \| H_{j}\|_{Q,2}, \s{H}_{j}, L_2(Q) \right)\sup_Q N\left(\varepsilon \| H_r\|_{Q,2}, \Lambda_r, L_2(Q) \right) \label{eq1:product_covering}
\end{align}
for any $\varepsilon > 0$ relative to the envelope function of each classes, $H_{h,s,j}$, $H_{h}$, $H_{j}$ and $H_{r}$. We now provide upper bounds for the uniform entropy separately. 

For the first class, we define the envelop function as a constant function $H_h := a \mapsto (\log n / h)^{1/2} \|K\|_\infty$ and thus we have
\[\sup_Q\| H_{h}\|_{Q,2} \geq \| H_{h}\|_{P,2} = \left( \frac{\log n}{h}\right)^{1/2}\|K\|_\infty.\]

This implies that the uniform entropy is bounded as follows;
\begin{align}
    \sup_Q N\left(\varepsilon \| H_{h}\|_{Q,2}, \s{H}_{h}, L_2(Q) \right) &\leq \sup_Q N\left(\varepsilon \left( \frac{\log n}{h}\right)^{1/2}\|K\|_\infty, \left( \frac{\log n}{h}\right)^{1/2}\tilde{\s{H}}_{h}, L_2(Q) \right) = \sup_Q N\left(\varepsilon \|K\|_\infty, \tilde{\s{H}}_{h}, L_2(Q) \right) \nonumber 
\end{align}
where $\tilde{\s{H}}_{h} := \left\{K\left(\frac{a-s}{h}\right) : s \in \s{S}\right\}.$ The last term is simply the uniform entropy of the class $\tilde{\s{H}}_{h}$ since its envelope function is given by the constant $\|K\|_\infty$. This class is VC type under \ref{cond:bounded_K} based on the result of \cite{gine2002}. Finally, Theorem 2.6.7 of \cite{vandervaart1996} states that for any probability measure $Q$, 
\[N\left(\varepsilon \| H_{h}\|_{Q,2}, \s{H}_{h}, L_2(Q) \right)\lesssim  \varepsilon^{-2(V(\s{H}_h)-1)}\]
where $V(\s{H}_h)$ is VC-index of the set of subgraphs of functions in $\s{H}_j$.

Next we provide the bound for the second term of (\ref{eq1:product_covering}). We first note that each function in $\s{H}_j$ satisfies the following composition: $u \mapsto u^jI\left(|u| \leq 1\right) = \phi \circ p_j(u)$ where $\phi := u \mapsto u I (|u| \leq 1)$ and $p_j := u \mapsto u^j$. Since $\phi$ is a bounded real function of a bounded variation and $p_j$ is a polynomial, the result from \cite{gine2002} implies that $\s{H}_j = \left\{ \phi \circ p_j\left(\frac{a-s}{h}\right) : s \in \s{S}\right\}$ is a bounded VC class of measurable functions. Then by using Theorem 2.6.7 of \cite{vandervaart1996} again, we have
\[N\left(\varepsilon \| H_{j}\|_{Q,2}, \s{H}_{j}, L_2(Q) \right)\lesssim  \varepsilon^{-2(V(\s{H}_j)-1)}\]
where $(V(\s{H}_j)$ is VC-index of the set of subgraphs of functions in $\s{H}_j$.

Finally, the uniform entropy of $\s{H}_r$ is certainly upper bounded by the the uniform entropy of $\Lambda$. By assumption, we have that
$\sup_Q \log N\left(\varepsilon \| H_r\|_{Q,2}, \Lambda_r, L_2(Q) \right) \lesssim \varepsilon^{-V}$ for $V < 2$. Plugging these results into equation (\ref{eq1:product_covering}) and taking log both sides, we get 
\[
    \sup_Q  \log N\left(\varepsilon \| H_{h,s,j}\|_{Q,2}, \s{H}_{h,s,r,j}, L_2(Q) \right) \lesssim \varepsilon^{-V}
\]
since the third term dominates the rest of them. 

Finally, we derive the bound on the uniform entropy integral of $\s{H}_{h,s,r,j}$, which can be evaluated as follows;
\begin{align*}
    J(\delta, \s{H}_{h,s,r,j},L_2) &= \sup_Q \int_0^\delta \sqrt{1 + \log  N\left(\varepsilon \| H_{h,s,j}\|_{Q,2}, \s{H}_{h,s,r,j}, L_2(Q) \right)} \, d\varepsilon \leq \int_0^\delta \sqrt{1 + C \varepsilon^{-V}} \, d\varepsilon \lesssim \int_0^\delta  \varepsilon^{-V/2} \, d\varepsilon  \lesssim \delta^{1-V/2}.
\end{align*}
\end{proof}

Derivation, for our records (store somewhere safe): Note that $1 / \sqrt{c - \log x} \leq 1 /\sqrt{c}$, and that 
\[\frac{d}{dx} [ x \sqrt{c - \log x}] = \sqrt{c - \log x} - \frac{1}{2\sqrt{c - \log x}}. \]
Hence,
\begin{align*}
    \int_0^t \sqrt{c - \log x} \, dx &\leq \int_0^t \left[\sqrt{c - \log x} - \frac{1}{2\sqrt{c - \log x}} + \frac{1}{2\sqrt{c}} \right] \, dx \\
    &= \int_0^t d\left[x\sqrt{c - \log x} \right] +\int_0^t \frac{1}{2\sqrt{c}} \, dx \\
    &= t\left[\sqrt{c - \log t} + 2 / \sqrt{c}\right].
\end{align*}
Therefore,
\begin{align*}
     \int_0^\delta \sqrt{1 -\frac{1}{2} \log h -2 \log \varepsilon} \, d\varepsilon &=  \sqrt{2}\int_0^\delta \sqrt{[1/2  -(\log h)/4] - \log \varepsilon} \, d\varepsilon \\
     &\leq   \sqrt{2} \delta \left[\sqrt{[1/2  -(\log h)/4] - \log \delta} + 2 / \sqrt{1/2  -(\log h)/4} \right] .
\end{align*}

\begin{lemma} If 
$E_0\left[\sup_{\eta \in \s{H}_{h,s,r,j}} \d{G}_n \eta\right] = \fasterthan(1)$
\end{lemma}
\begin{proof}[\textbf{Proof of Lemma}]

\end{proof}

We define the envelope function of $\s{H}_{h,s,r,j} := \{ \eta_{h,s, j,\lambda} : s \in \s{S}, \lambda \in \Lambda_r\}$ as 
\[H_{h,s,r,j} := (y, a, w) \mapsto (\log n/h)^{1/2} \|K\|_\infty \sup_{\lambda \in \Lambda_r}(\lambda-\lambda_\infty)(y, a, w)\]
\kt{We can define the envelope with $\bar{\Lambda}$. Thanks Ted!}
\[H_{h,s,r,j} := (y, a, w) \mapsto (\log n/h)^{1/2} \|K\|_\infty 2\bar{\Lambda}(y, a, w)\]
using the definition of $K$ from \ref{cond:bounded_K}. We also denote by $\bar{\Lambda}(y,a,w)$ the envelope for $\Lambda$ \kt{Will place conditions on this, most likely in terms of finite $P_{(4p-2)/(p-1)}$ norm}. Next we check following conditions in order to apply Theorem 3.1 of \cite{van2011local}. First, we note that
\begin{align*}
    P_0 H_{h,s,r,j}^{(4p-2)/(p-1)} &= (\log n/h)^{(2p-1)/(p-1)} \|K\|^{(4p-2)/(p-1)}_\infty \int \sup_{\lambda \in \Lambda_r} \{|\lambda - \lambda_\infty|\}^{(4p-2)/(p-1)} \, dP_0(z) \\
    &\leq (\log n/h)^{(2p-1)/(p-1)}  \|2\bar{\Lambda}\|^{(4p-2)/(p-1)}_{P_0,(4p-2)/(p-1)} < \infty.
\end{align*}

Next for each $\eta_{h,s,r,j} \in \s{H}_{h,s,r,j}$, we have that 
\begin{align*}
    P \eta^2_{h,s,r,j} &= \int \left\{(h\log n)^{1/2} \left(\frac{a-s}{h}\right)^{j-1}K_{h,s}(a) (\lambda-\lambda_\infty)(y, a, w)\right\}^2\, dP_0(z) \\
    &= \log n \int u^{2(j-1)}K^2(u)E_0[(\lambda-\lambda_\infty)^2 \mid A=s+uh] f_0(s+uh) \, du \\
    &\leq r^2 \log n  \int u^{2(j-1)}K^2(u)f_0(s+uh) \, du.
\end{align*}
In contrast, for $H_{h,s,r,j}$, we have that 
\begin{align*}
    P H^2_{h,s,r,j} &= \int \left\{(\log n/h)^{1/2} \|K\|_\infty \sup_{\lambda \in \Lambda_r}(\lambda-\lambda_\infty)(y, a, w)\right\}^2\, dP_0(z) \\
    &\leq  \frac{\log n}{h} \|K\|_\infty^2 \|2\bar{\Lambda}\|_{P_0, 2}^2. 
\end{align*}

This implies the relationship $P \eta^2_{h,s,r,j} < hr^2  P H^2_{h,s,r,j}$. We now use Theorem 3.1 of \cite{van2011local}, which states that
% \begin{align}
%     E_0 \left[\sup_{\eta \in \s{H}_{h,s,r,j}} |\d{G}_n \eta|\right] \lesssim J(h^{1/2}, \s{H}_{h,s,r,j}, L_2)\left(\underbrace{1}_\text{(I)}+\underbrace{\frac{J(h^{1/2p}, \s{H}_{h,s,r,j}, L_2)}{h\sqrt{n}\left(P H^2_{h,s,r,j}\right)^{1-1/2p}}}_\text{(II)}\right)^{p/(2p-1)} \left(P H^2_{h,s,r,j}\right)^{1/2}
% \end{align}
\begin{align}
    E_0 \left[\sup_{\eta \in \s{H}_{h,s,r,j}} |\d{G}_n \eta|\right] \lesssim J(rh^{1/2}, \s{H}_{h,s,r,j}, L_2)\left(\underbrace{1}_\text{(I)}+\underbrace{\frac{J(r^{1/p}h^{1/2p}, \s{H}_{h,s,r,j}, L_2)\left(P H^{(4p-2)/(p-1)}_{h,s,r,j}\right)^{(p-1)/2}}{hr^2\sqrt{n}\left(P H^2_{h,s,r,j}\right)^{1-1/2p}}}_\text{(II)}\right)^{p/(2p-1)} \left(P H^2_{h,s,r,j}\right)^{1/2}
\end{align}
In the following analysis, we assume that $h = \boundeddet(n^{-1/5})$. We first show when the term $(II)$ diverges since it changes the dominating terms. By Lemma \ref{lm:uniform_entropy}, we have

$J(\delta, \s{H}_{h,s,r,j}, L_2) \leq \delta^{1-V/2}$ and thus, 
% \begin{align*}
%     \frac{J(h^{1/2p}, \s{H}_{h,s,r,j}, L_2)}{h\sqrt{n}\left(P H^2_{h,s,r,j}\right)^{1-1/2p}} &\leq 
%     \frac{h^{1/2p-V/4p}}{h\sqrt{n}\left( r^2 \frac{\log n}{h} \right)^{1-1/2p}} = \frac{h^{-V/4p}}{\sqrt{n}\left( r^2 \log n \right)^{1-1/2p}} = \frac{n^{V/20p-1/2}}{n ^{(1/2p-1)c}}.
% \end{align*}
\begin{align*}
    \frac{J(r^{1/p}h^{1/2p}, \s{H}_{h,s,r,j}, L_2)\left(P H^{(4p-2)/(p-1)}_{h,s,r,j}\right)^{(p-1)/2}}{hr^2\sqrt{n}\left(P H^2_{h,s,r,j}\right)^{1-1/2p}} &\leq 
    \frac{r^{1/p-V/2p}h^{1/2p-V/4p}\left( \frac{\log n}{h} \right)^{(2p-1)/2}}{hr^2\sqrt{n}\left( \frac{\log n}{h} \right)^{1-1/2p}} \\
    &=\frac{r^{1/p-V/2p-2}h^{-V/4p-(2p-1)/2}\left( \log n \right)^{p+1/2p-3/2}}{\sqrt{n}} \\
    &=r^{\frac{2-V}{2p}-2}\frac{\left( \log n \right)^{p+1/2p-3/2}}{n^{3/10-V/20p}}
\end{align*}
\kt{Since $p > 1$ and $V < 2$, it implies $\frac{2-V}{2p}-2 < 0$. (II) dominates when this term diverges. When it doesn't, the restriction on $V$ and $r$ becomes too string (i.e., see below) so I think we want this term to diverge. The denominator grows at $n^{3/10}$ or slower so letting this term diverge is easier. But if it's too fast, controlling the overall term becomes difficult. We can't let $p$ grow too big either due to $(\log n)^p$ term (unless $r = n^{-p}$ but this is again too strong).}

\begin{align*}
    \frac{J(r^{1/p}h^{1/2p}, \s{H}_{h,s,r,j}, L_2)\left(P H^{(4p-2)/(p-1)}_{h,s,r,j}\right)^{(p-1)/2}}{hr^2\sqrt{n}\left(P H^2_{h,s,r,j}\right)^{1-1/2p}} &\lesssim \frac{ r^{\frac{1-V/2}{p}} h^{\frac{1-V/2}{2p} - \frac{2p-1}{2}} (\log n)^{\frac{2p-1}{2}} }{r^2 h^{1-(1-1/2p)} \sqrt{n} (\log n)^{1-1/2p}} \\
    &= r^{1/p - V/(2p) - 2} h^{1/2 - p - V / (4p)} n^{-1/2}(\log n)^{p + 1/(2p) - 3/2}
\end{align*}
$1/p - V/(2p) - 2 \in (-2, -1)$. $1/2 - p - V/(4p) \in (-\infty, -1/2)$. If $h=n^{-1/5}$ then the above equals
\[ r^{1/p - V/(2p) - 2} n^{\frac{V/(4p) + p - 3}{5}} (\log n)^{p + 1/(2p) - 3/2} = \left( r n^{\frac{V/2 + 2p^2 - 6p}{5(2 - V - 4p)}}(\log n)^{\frac{1 + 2p^2 - 3p}{2 - V - 4p}}\right)^{1/p - V/(2p) - 2}\]
This goes to $\infty$ if and only if 
\[ r = \fasterthandet\left( n^{-\frac{V/2 + 2p^2 - 6p}{5(2 - V - 4p)}}(\log n)^{-\frac{1 + 2p^2 - 3p}{2 - V - 4p}}\right)\]
Regime change occurs at $p > (3 + \sqrt{9-V})/2$. Then the expression is always going to $\infty$ as long as $r$ goes to zero, I think. Otherwise it depends on rate of $r$. 

IF $p > (3 + \sqrt{9-V})/2$ (which holds for sure if $p > 3$ so $|Y|$ has finite $5+\delta$ moment) or $r$ is slower than what is above, then I believe the rate is 
\[  J(rh^{1/2}, \s{H}_{h,s,r,j}, L_2) \left(P H^2_{h,s,r,j}\right)^{1/2} = r^{1-V/2} h^{-V/4} (\log n)^{-1/2}.\]
Up to log terms, we need the rate to be $r = o(h^{\frac{V/4}{1-V/2}})$. For $V = 1$ and $h = n^{-1/5}$ this is $n^{-1/10}$ which is reasonable. As $V$ gets closer to 2, gets worse.
